# Supplementary material for: Protection of quantum information in a chain of Josephson junctions
Source: arXiv:2205.13929 source file (2022-05-27)
Supplement: Supplementary file 1 [file supplementary_from_paul_1.tex]

\setcounter{page}{1}

\section*{Supplementary Material}

\subsection*{Disorder}

In order to model the effect of disorder on our qubit we vary the junction charging and tunneling energies, loop areas and gate charges as described in the main body of the text. In Fig. \ref{fig:junction_disorder} we display the effect of $2 \%$ disorder in the junction parameters and we find the good performance of the qubit is retained.

In Fig. \ref{fig:loop_disorder} we turn our attention to disorder in the loops of the circuit by introducing a $0.2 \%$ variation in their sizes. Such disorder does not affect the charge noise dephasing time, so we only display the flux noise dephasing time and the gap of the qubit. We find that our design is robust to this level of disorder with no significant change in the gap and even a slight improvement in flux dephasing time.

Finally in Fig. \ref{fig:gate_disorder} we introduce gate charge disorder at a level of $0.1 \%$. This kind of disorder does not affect the flux noise dephasing time so we only display the charge noise dephasing time, which now varies significantly. However, the dephasing time remains in the millisecond range and the gap is almost unaffected.

\begin{figure*}[h]
\centering
\includegraphics[width=\linewidth]{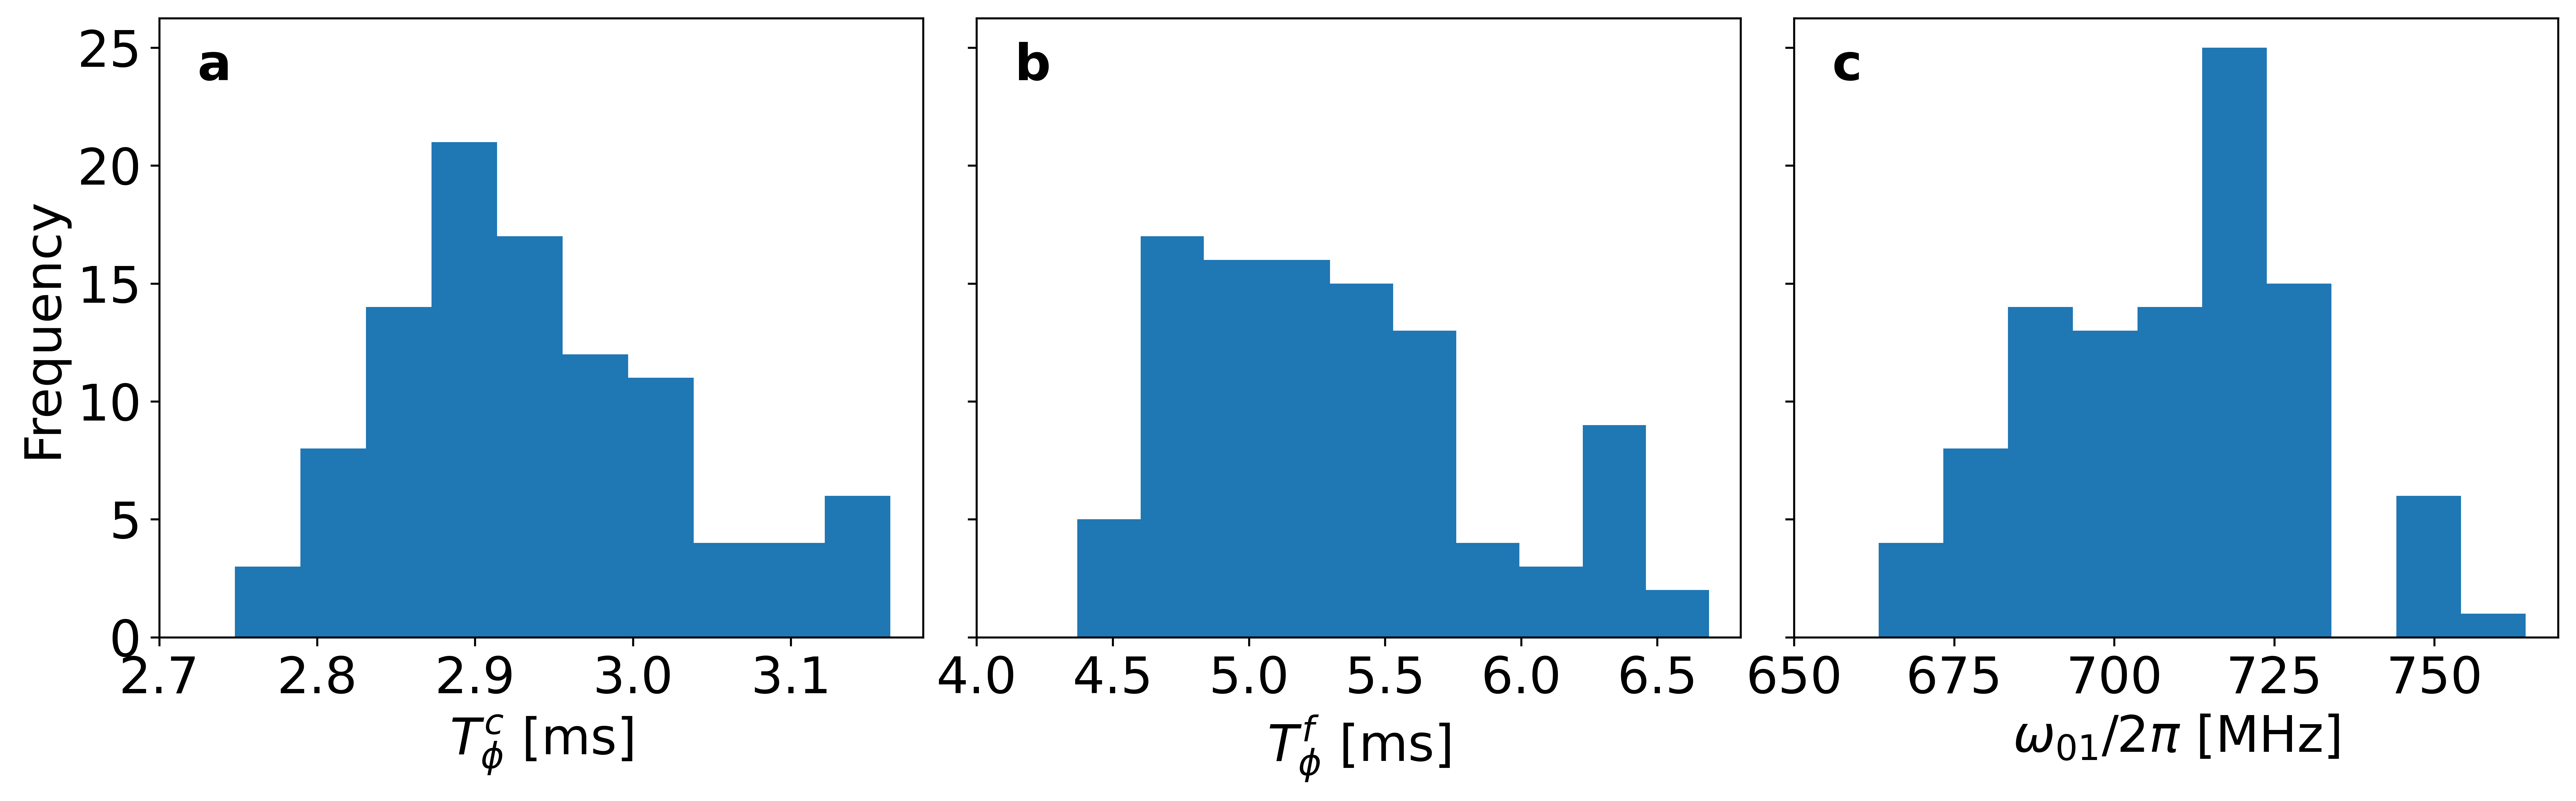}
\caption{\textbf{Junction disorder.} We introduce a $2 \%$ variation in the sizes and oxidation parameters of the junctions and plot histograms of the resulting variations in (\textbf{a}) the charge dephasing time $T^c_\phi$, (\textbf{b}) the flux dephasing time $T^f_\phi$ and (\textbf{c}) the gap of the qubit $\omega_{01}/2\pi$. The resulting expectation values and standard deviations of these characteristics are (\textbf{a}) $2.94 \pm 0.10 ~\mathrm{ms}$, (\textbf{b}) $5.32 \pm 0.54 ~\mathrm{ms}$ and (\textbf{c}) $708 \pm 21 ~\mathrm{MHz}$ respectively. This level of disorder creates no significant degradation in the qualities of the qubit. }\label{fig:junction_disorder}
\end{figure*}

\begin{figure*}[h]
\centering
\includegraphics[width=\linewidth]{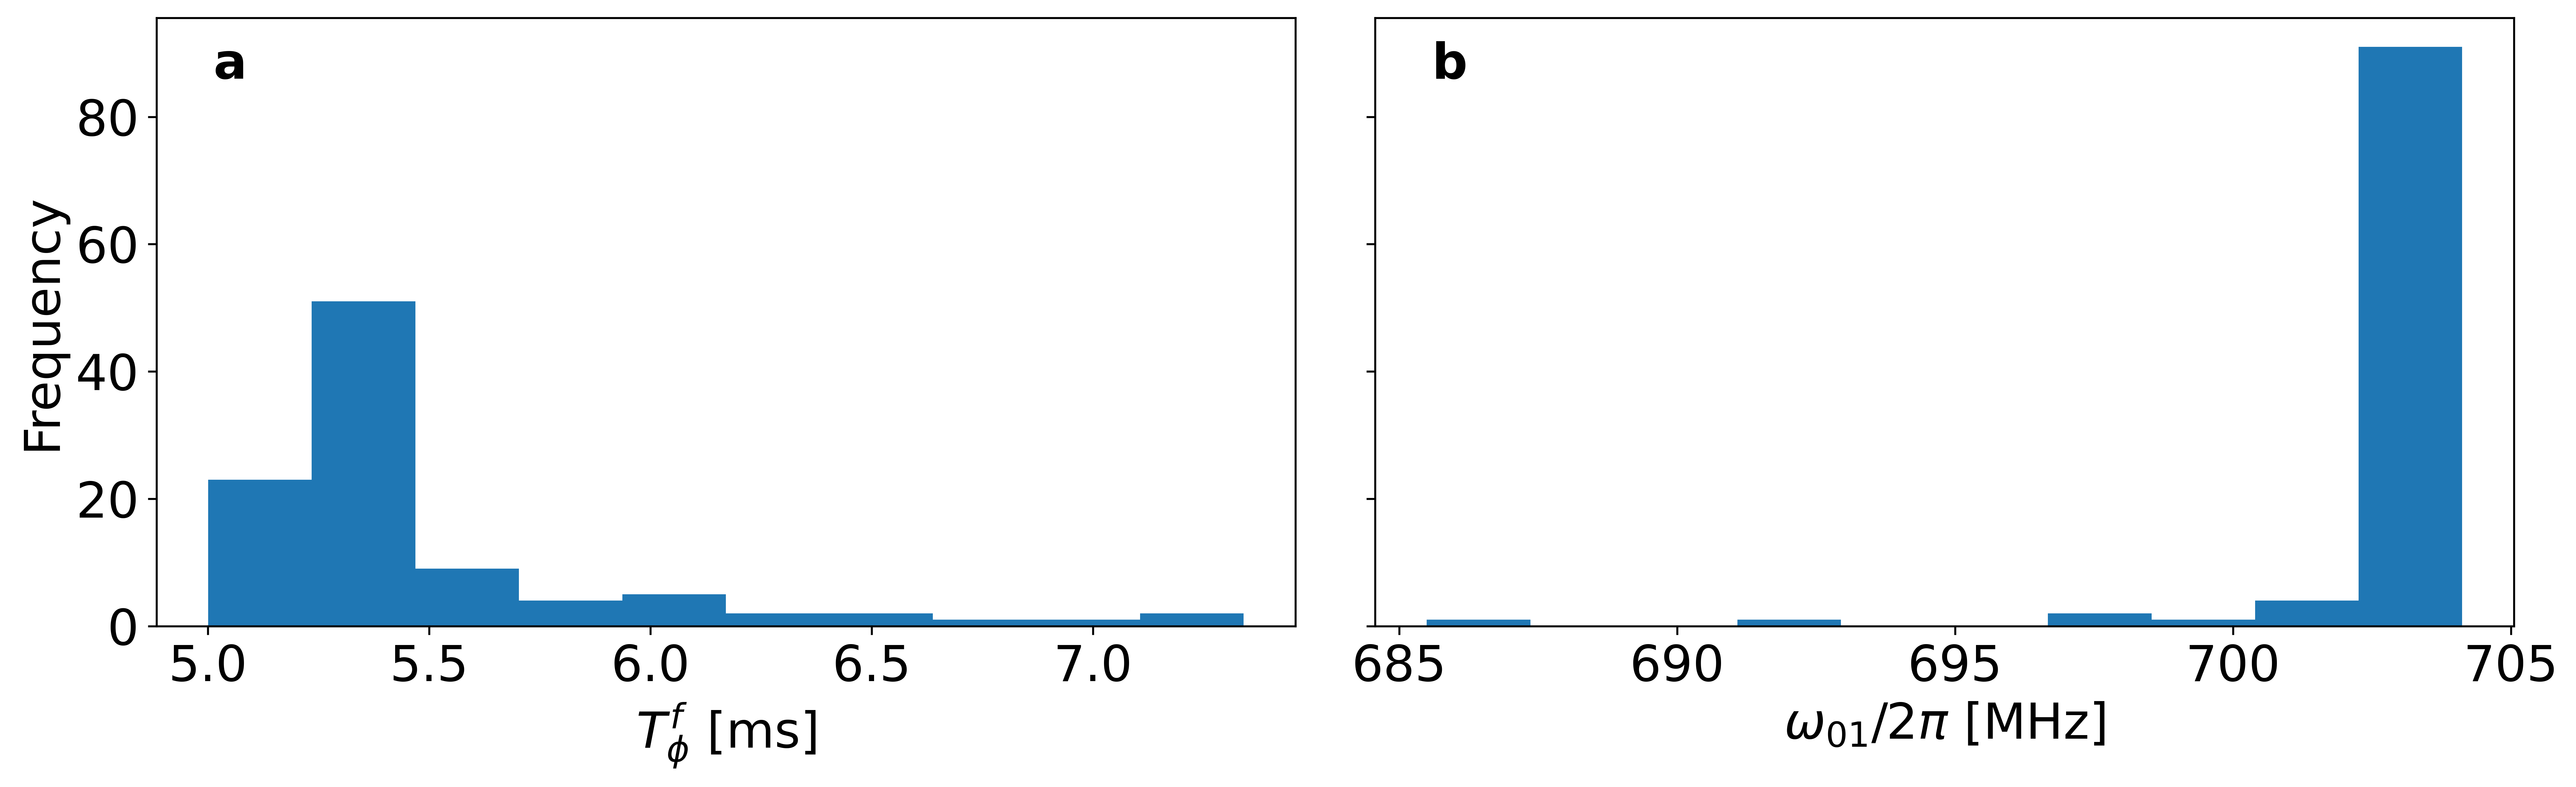}
\caption{\textbf{Loop disorder.} We introduce a $0.2 \%$ variation in the sizes of the loops and plot histograms of the resulting variations in (\textbf{a}) the flux dephasing time $T^f_\phi$ and (\textbf{b}) the gap of the qubit $\Delta \omega_{01}/2\pi$. The resulting expectation values and standard deviations of these characteristics are (\textbf{a}) $5.45 \pm 0.46 ~\mathrm{ms}$ and (\textbf{b}) $703 \pm 2 ~\mathrm{MHz}$ respectively. This level of disorder creates no significant degradation in the qualities of the qubit. }\label{fig:loop_disorder}
\end{figure*}

\begin{figure*}
\centering
\includegraphics[width=\linewidth]{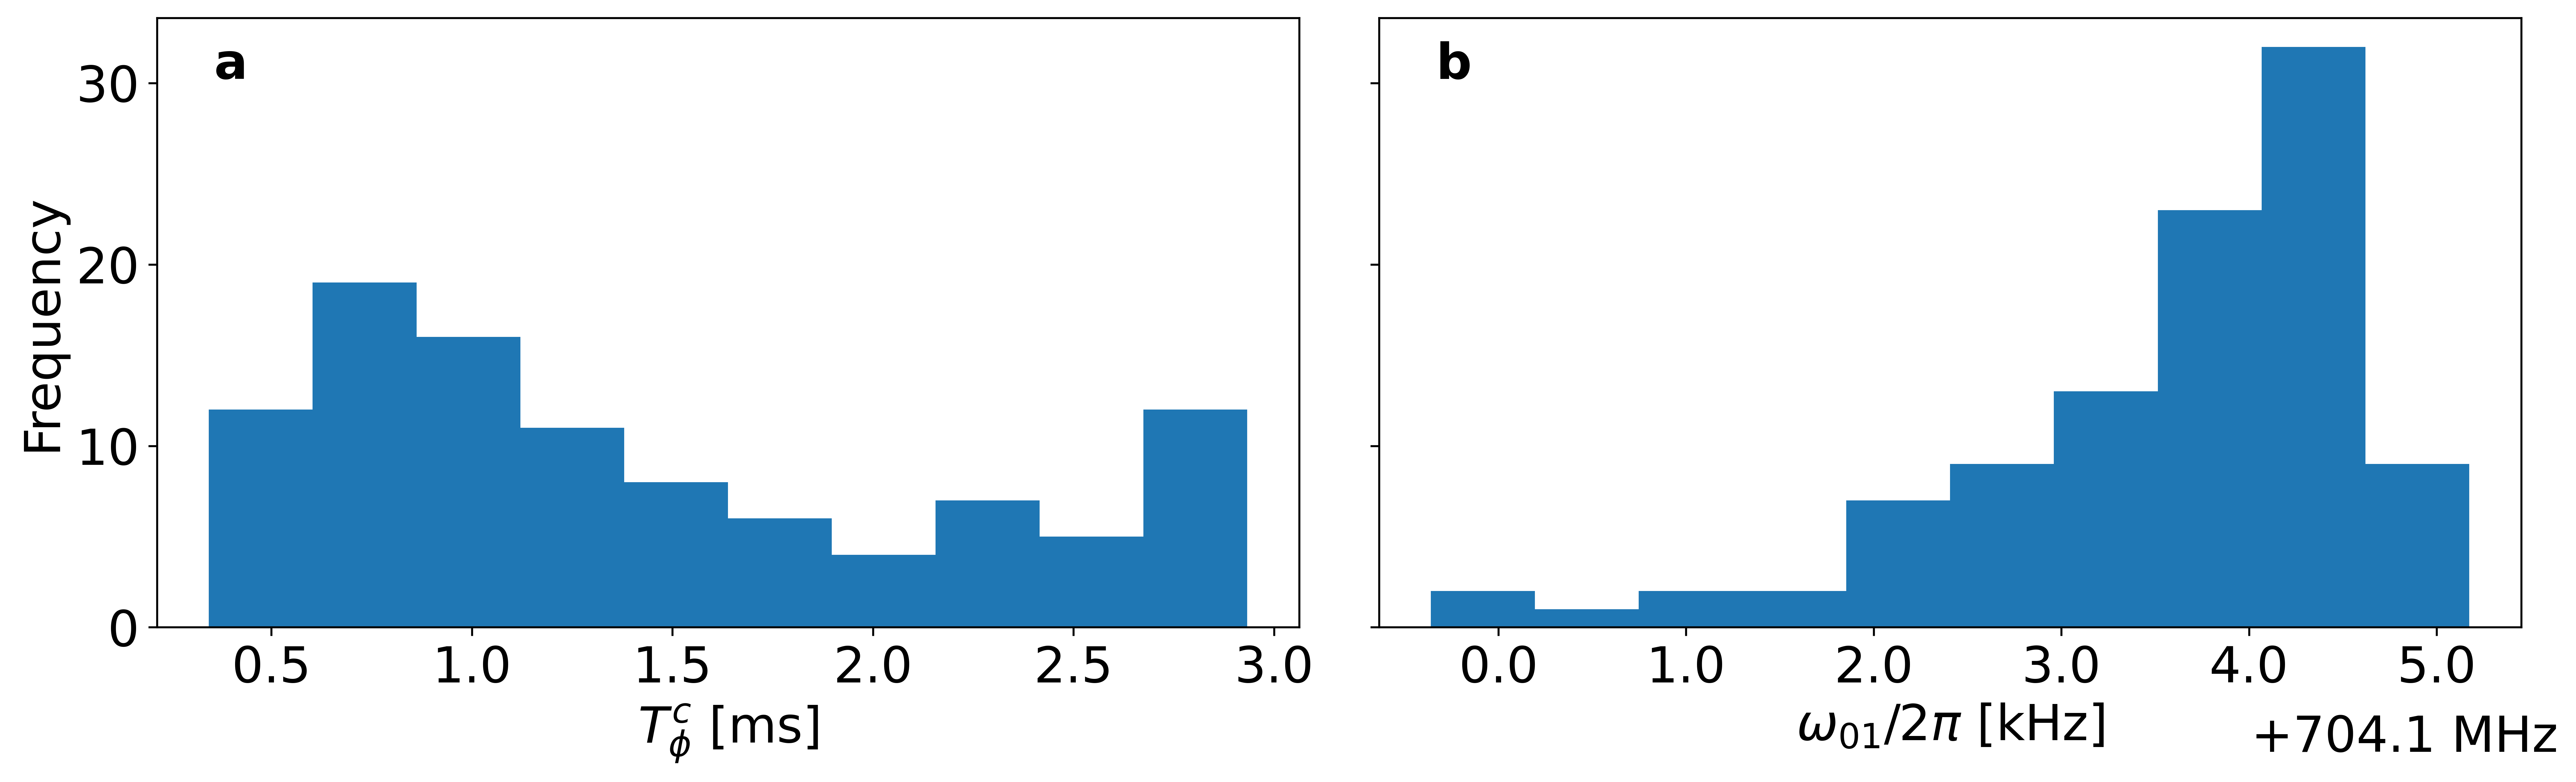}
\caption{\textbf{Gate disorder.} We introduce a $0.1 \%$ variation in the gate charges and plot histograms of the resulting variations in (\textbf{a}) the charge dephasing time $T^c_\phi$ and (\textbf{b}) the gap of the qubit $\Delta \omega_{01}/2\pi$. The resulting expectation values and standard deviations of these characteristics are (\textbf{a}) $1.44 \pm 0.78 ~\mathrm{ms}$ and (\textbf{b}) $704.103 \pm 0.001 ~\mathrm{MHz}$ respectively. This level of disorder reduces the coherence time of the qubit but leaves the gap unchanged. }\label{fig:gate_disorder}
\end{figure*}
